# Supplementary material for: Band-limited Training and Inference for Convolutional Neural Networks
Source: arXiv:1911.09287 source file (2019-11-21)
Supplement: Supplementary file 1 [file additional_results.tex]

\section{Additional results}

\subsection{Training with compression for convolution}
\begin{figure}[t]                                                                                                                                                                                                           
  \centering                                                                                                                                                                                                                
  \includegraphics[width=\linewidth]{cifar10initial2.pdf} % width=\linewidth]
  \caption{{\it Training accuracy with different types of convolutional layers and applying various compression ratios.}}                                  
  \label{fig:compareCompressionSmall}                                                                                                                                                                                             
\end{figure}
The only difference in the configuration between training presented in Figure~\ref{fig:compareCompressionSmall} and the one presented in Figure~\ref{fig:500epochs} is the size of the stride for max pool layers.

\subsection{Crossover between direct and FFT based convolution}

\begin{figure}[t]                                                                                                                                                                                                           
  \centering                                                                                                                                                                                                                
  \includegraphics[width=\linewidth]{scipyCrossover.png} % width=\linewidth]
  \caption{{\it The crossover point between direct and FFT based 1D convolution.}}                                  
  \label{fig:crossoverScipy}
\end{figure}

In Figure~\ref{fig:crossoverScipy}, for SciPy the input signal size is 4096 values, we change the size of the filter from 1 to 2048 values, for the filter size of about 300 values. we observe the cross-over point: for filters of size fewer than 300 values, direct convolution is faster, for filters larger than 300, the FFT based convolution is faster.

\begin{figure}[t]                                                                                                                                                                                                           
  \centering                                                                                                                                                                                                                
  \includegraphics[width=\linewidth]{similarShape.png} % width=\linewidth]
  \caption{{\it Similar shape of time series data before and after compression in the frequency domain.}}                                  
  \label{fig:similarShape}
\end{figure}

\begin{figure}[t]                                                                                                                                                                                                        
  \centering                                                                                                                                                                                                                
  \includegraphics[width=\linewidth]{crossCorelation2D-2.png} % width=\linewidth]
  \caption{{\it Cross-correlation in 2D with FFTW, PyTorch on CPU and GPU, naive FFT, scipy FFT.}}                                  
  \label{fig:crossCorrelation2D}
\end{figure}

\subsection{DTW for time-series}
We also try to leverage other techniques from speech technologies in the analysis of time series data. The initial experiments with DTW for time-series suggest that it can provide results of good accuracy, but its implementation in Python is running rather very slowly (for some datasets with long time-series and a single template for DTW, it can run a few hours).
